# Supplementary material for: Intrinsic Pulsed Magnetic Gradiometer in Earth's Field
Source: arXiv:2111.12310 source file (2021-11-24)
Supplement: Supplementary file 1 [file Supplimental2.pdf]

# Spatial Evolution of The Multi-Coherent Light in Alkali-Metal Vapor

Yuan-Yu Jau

June 12, 2007

## Starting from Maxwell's equations

Maxwell equations in cgs unit state

$$\begin{aligned}
\nabla \cdot \mathbf{D}_e &= 4\pi\rho, \\
\nabla \cdot \mathbf{B} &= 0, \\
\nabla \times \mathbf{E} &= -\frac{1}{c}\frac{\partial \mathbf{B}}{\partial t}, \\
\nabla \times \mathbf{H} &= \frac{1}{c}\frac{\partial \mathbf{D}_e}{\partial t} + \frac{4\pi}{c}\mathbf{J}.
\end{aligned} \tag{1}$$

Of our interest, we look at the case of no spatial charge $\rho \approx 0$, no current source $\mathbf{J} \approx 0$, and no magnetic susceptibility $\mathbf{B} \approx \mathbf{H}$. Therefore, we can find

$$\nabla \times \nabla \times \mathbf{E} = -\nabla^2 \mathbf{E} + \nabla(\nabla \cdot \mathbf{E}) = -\frac{1}{c^2}\frac{\partial^2 \mathbf{D}_e}{\partial t^2}. \tag{2}$$

The electrical displacement density $\mathbf{D}_e$ has connection with induced electric dipoles $\langle \mathbf{D} \rangle = \langle \mathbf{D}(t, \mathbf{r}) \rangle$ of alkali-metal atoms, and we find

$$\mathbf{D}_e = \mathbf{E} + 4\pi \mathbf{P} = \mathbf{E} + 4\pi n_a \langle \mathbf{D} \rangle. \tag{3}$$

Here, $n_a$ is the number density of alkali-metal atoms. The induced dipole is calculated by

$$\langle \mathbf{D}(t, \mathbf{r}) \rangle = \int \langle \boldsymbol{\alpha}(t, \omega) \rangle_\rho \widetilde{\mathbf{E}}(\omega, \mathbf{r}) e^{-i\omega t} d\omega. \tag{4}$$

The expectation value of the polarizability, $\boldsymbol{\alpha}$, of the atoms is

$$\langle \boldsymbol{\alpha}(t, \omega) \rangle_\rho = \mathrm{Tr}(\rho(t, \mathbf{r}) \boldsymbol{\alpha}(\omega)), \tag{5}$$

and the matrix elements of $\boldsymbol{\alpha}$ are

$$\boldsymbol{\alpha}_{\mu\nu}(\omega) = \frac{1}{\hbar} \sum_{\bar{\mu}} \frac{\mathbf{D}_{\mu\bar{\mu}} \mathbf{D}^\dagger_{\bar{\mu}\nu}}{(\omega_{\bar{\mu}\nu} - \omega) - i\gamma_{\bar{\mu}\nu}}. \tag{6}$$

Here, the dipole operator, $\mathbf{D}$, is defined by

$$\mathbf{D}_{\mu\bar{\mu}}\mathbf{D}^{\dagger}_{\bar{\mu}\nu} = \frac{\hbar r_e c^2 f}{\omega_{\bar{\mu}\nu}}\mathbf{A}_{\mu\bar{\mu}}\mathbf{A}^{\dagger}_{\bar{\mu}\nu}, \tag{7}$$

and the transition operator, $\mathbf{A}$, can be expressed by using spherical tensor $T_{\alpha\beta}$ as

$$\mathbf{A} = \sum_{\sigma} \xi^*_{\sigma} T_{1\sigma}(J\bar{J}), \tag{8}$$

where $\xi_\sigma$ is the spherical basis. For convenience, the electric field can be expressed as the sum of all frequency components. Hence,

$$\mathbf{E}(t,\mathbf{r}) = \int \widetilde{\mathbf{E}}(\omega,\mathbf{r})e^{-i\omega t}d\omega. \tag{9}$$

Since the physical electric field contains both the positive-frequency components and their complex conjugate parts, due to the symmetry, it is sufficient to consider only a complex electric field with positive-frequency components. We define

$$\widetilde{\mathbf{E}}(\omega,\mathbf{r})|_{\omega<0} = 0. \tag{10}$$

Because we are interested in static light propagation, we carrier out the time derivative by using Eq. (9) and Eq. (4) to get rid of the time-dependent part in Eq. (2) , and we find

$$\nabla^2\widetilde{\mathbf{E}} - \nabla(\nabla\cdot\widetilde{\mathbf{E}}) = -\frac{\omega^2}{c^2}\left(\widetilde{\mathbf{E}} + 4\pi n_a\langle\widetilde{\mathbf{D}}\rangle\right), \tag{11}$$

where

$$\langle\mathbf{D}(t,\mathbf{r})\rangle = \int \langle\widetilde{\mathbf{D}}(\omega,\mathbf{r})\rangle e^{-i\omega t}d\omega. \tag{12}$$

## Vector representation of electric field

Considering the electric field as a vector, therefore

$$\mathbf{E} = \sum_{\omega\geq 0}\widetilde{\mathbf{E}}_\omega|\omega\rangle e^{-i\omega t}, \text{ and } \widetilde{\mathbf{E}} = \sum_{\omega\geq 0}\widetilde{\mathbf{E}}_\omega|\omega\rangle. \tag{13}$$

Here, $|\omega\rangle$ is the electric field basis labelled with optical frequency $\omega$, and $\langle\omega'|\omega\rangle = \delta_{\omega',\omega}$. By using Eq. (11) and Eq. (13), we find

$$\nabla^2\widetilde{\mathbf{E}} - \nabla(\nabla\cdot\widetilde{\mathbf{E}}) = -\frac{\mathbf{W}^2}{c^2}\cdot(1+\boldsymbol{\chi})\cdot\widetilde{\mathbf{E}}. \tag{14}$$

Here, $\mathbf{W}$ is the dyadic frequency matrix, where $\langle\omega'|\mathbf{W}|\omega\rangle = \omega'\boldsymbol{\delta}_{\omega',\omega}$, and $\boldsymbol{\chi}$ is the dyadic electric susceptibility operator, where

$$\langle\omega'|\boldsymbol{\chi}|\omega\rangle = 4\pi n_a \sum_{\mu,\nu}\boldsymbol{\alpha}_{\mu\nu}\tilde{\rho}_{\mu\nu}\delta_{(\omega'-\omega),\Omega_{\mu\nu}}e^{\frac{i}{c}(\omega'-\omega)z}. \tag{15}$$

The density-matrix amplitude, $\tilde{\rho}_{\mu\nu}$, is defined by

$$\rho_{\mu\nu} = \tilde{\rho}_{\mu\nu} e^{-i\Omega_{\mu\nu} t}, \tag{16}$$

where $\Omega_{\mu\nu} t \approx (\omega_\mu - \omega_\nu)t$ is the excited time-dependent phase due to the external causes, such as RF fields, modulated light, etc.

Considering one-dimensional plane wave along the z-direction, we can find $\nabla^2 \widetilde{\mathbf{E}} - \nabla(\nabla \cdot \widetilde{\mathbf{E}}) \longrightarrow \frac{\partial^2}{\partial z^2}\widetilde{\mathbf{E}}$, therefore Eq. (14) can be approximated as

$$\left(\frac{\partial}{\partial z} \pm i\frac{\mathbf{W}}{c} \cdot \sqrt{1+\boldsymbol{\chi}}\right) \cdot \widetilde{\mathbf{E}}_\pm = 0. \tag{17}$$

For most of cases, $|\boldsymbol{\chi}| \ll 1$, so $\sqrt{1+\boldsymbol{\chi}} \approx 1 + \boldsymbol{\chi}/2$, and therefore we find

$$\left(\frac{\partial}{\partial z} \pm i\frac{\mathbf{W}}{c} \cdot (1+\boldsymbol{\chi}/2)\right) \cdot \widetilde{\mathbf{E}}_\pm = \left(\frac{\partial}{\partial z} \pm \frac{i}{\hbar}\left(\mathbf{P_0} + \boldsymbol{\delta}\mathbf{P}\right)\right) \widetilde{\mathbf{E}}_\pm = 0. \tag{18}$$

Here, the subscript $\pm$ represents the electric fields of forward and backward propagations, and the two dyadic momentum operators $\mathbf{P_0}$ and $\boldsymbol{\delta}\mathbf{P}$ are found to be

$$\langle \omega' | \mathbf{P_0} | \omega \rangle = \frac{\hbar \mathbf{W}}{c} = \hbar k' \boldsymbol{\delta}_{\omega',\omega},\ k' = \frac{\omega'}{c},\ k = \frac{\omega}{c}, \tag{19}$$

and

$$\langle \omega' | \boldsymbol{\delta}\mathbf{P} | \omega \rangle = \frac{\hbar \mathbf{W}}{c} \cdot \frac{\boldsymbol{\chi}}{2} = \frac{4\pi n_a \hbar \omega'}{2c} \sum_{\mu,\nu} \boldsymbol{\alpha}_{\mu\nu} \tilde{\rho}_{\mu\nu} \delta_{(\omega'-\omega),\Omega_{\mu\nu}} e^{i(k'-k)z}. \tag{20}$$

The total electric field is $\widetilde{\mathbf{E}} = \widetilde{\mathbf{E}}_+ + \widetilde{\mathbf{E}}_-$.

## Density-matrix representation of electric field

Similar to alkali-metal atoms, we can describe electric field as a dyadic density matrix, $\boldsymbol{\epsilon}$.

$$\boldsymbol{\epsilon} = \frac{1}{S}\int_S \widetilde{\mathbf{E}}\widetilde{\mathbf{E}}^* da = \sum_{\omega',\omega} \boldsymbol{\epsilon}_{\omega'\omega} |\omega'\rangle\langle\omega|. \tag{21}$$

Here, we have $\mathrm{Tr}(\boldsymbol{\epsilon}) = \widetilde{\mathbf{E}} \cdot \widetilde{\mathbf{E}}^* = \sum_{\omega \geq 0} |\widetilde{\mathbf{E}}_\omega|^2$. In practice, for light detection, we have to integrate the cross area of the light beam. Due to the spatial modes, different positions on the cross area can have different phases, which cause spatial decoherence. From Eq. (18), we find the spatial evolution equation of electric-field density matrix, $\boldsymbol{\epsilon}$, to be

$$\frac{d}{dz}\boldsymbol{\epsilon}_\pm = \pm\frac{i}{\hbar}[\mathbf{P_0}, \boldsymbol{\epsilon}_\pm] \pm \frac{i}{\hbar}[\boldsymbol{\delta}\boldsymbol{\mathcal{E}}_\mathbf{o}, \boldsymbol{\epsilon}_\pm] \mp \frac{1}{2}\{\boldsymbol{\delta}\boldsymbol{\Gamma}_\mathbf{o}, \boldsymbol{\epsilon}_\pm\}. \tag{22}$$

Here, the Hermitian spatial-frequency-shift operator is

$$\boldsymbol{\delta}\boldsymbol{\mathcal{E}}_\mathbf{o} = \frac{1}{2}(\boldsymbol{\delta}\mathbf{P} + \boldsymbol{\delta}\mathbf{P}^\dagger), \tag{23}$$

and the Hermitian light absorption operator is

$$\boldsymbol{\delta\Gamma_o} = \frac{1}{i\hbar}(\boldsymbol{\delta}\mathbf{P} - \boldsymbol{\delta}\mathbf{P}^\dagger). \tag{24}$$

Again, we use the subscript $\pm$ to denote forward and backward parts, and $\boldsymbol{\epsilon} = \boldsymbol{\epsilon}_+ + \boldsymbol{\epsilon}_-$. In Eq. (22), the commutation and anti-commutation are defined by

$$[\mathbf{A}, \mathbf{B}] = \mathbf{A}\cdot\mathbf{B} - \mathbf{B}\cdot\mathbf{A} \text{ and } \{\mathbf{A}, \mathbf{B}\} = \mathbf{A}\cdot\mathbf{B} + \mathbf{B}\cdot\mathbf{A}. \tag{25}$$

## Duality of photons and alkali-metal atoms

Analogous to alkali-metal atoms, considering the case of only depopulation pumping, the evolution equation of the density matrix is

$$\frac{d}{dt}\rho = \frac{1}{i\hbar}[H_0, \rho] + \frac{1}{i\hbar}[\delta\mathcal{E}, \rho] - \frac{1}{2}\{\delta\Gamma, \rho\}, \tag{26}$$

and

$$\delta\mathcal{E} = \frac{1}{2}(\delta H + \delta H^\dagger), \text{ and } \delta\Gamma = \frac{i}{\hbar}(\delta H - \delta H^\dagger). \tag{27}$$

For comparison, $H_0$ of Eq. (26), an energy operator, defines the unperturbed time-dependent phase of $\rho$; and $\mathbf{P_0}$, a momentum operator, of Eq. (22) defines the unperturbed space-dependent phase of $\boldsymbol{\epsilon}$. As for the effective Hamiltonian $\delta H$ of atoms, we find

$$\langle\mu|\delta H|\nu\rangle = -\sum_{\omega',\omega} \frac{4\pi n_p \hbar\omega'}{2} \boldsymbol{\alpha}_{\mu\nu}(\omega) : \boldsymbol{\varepsilon}_{\omega'\omega} \delta_{(\omega'-\omega),\Omega_{\mu\nu}} e^{-i(\omega'-\omega)t}. \tag{28}$$

Here, $n_p = \sum_{\omega\geq 0} |\widetilde{\mathbf{E}}_\omega|^2/(2\pi\hbar\omega)$ is the photon density, and $\boldsymbol{\varepsilon} = \boldsymbol{\epsilon}/|\widetilde{\mathbf{E}}|^2$ is the normalized $\boldsymbol{\epsilon}$. Comparing with the effective spatial Hamiltonian $\boldsymbol{\delta}\mathbf{P}$ of photons, we have

$$\langle\omega'|\boldsymbol{\delta}\mathbf{P}|\omega\rangle = \sum_{\mu,\nu} \frac{4\pi n_a \hbar\omega'}{2c} \boldsymbol{\alpha}_{\mu\nu}(\omega) \tilde{\rho}_{\mu\nu} \delta_{(\omega'-\omega),\Omega_{\mu\nu}} e^{i(k'-k)z}. \tag{29}$$

One can easily point out the identity of Eq. (22) and Eq. (26), and also the similarity between Eq. (28) and Eq. (29). The spatial evolution of photons is identical to the temporal evolution of atoms. The polarizability operator $\boldsymbol{\alpha}$ plays a key role of the interaction between photons and atoms. By using Eq.(28) and Eq.(29), we can verify

$$\begin{aligned} c n_p \mathrm{Tr}(\boldsymbol{\delta\Gamma_o}\cdot\boldsymbol{\varepsilon}) &= n_a \mathrm{Tr}(\delta\Gamma\rho). \\ \text{(total photon absorption rate)} &= \text{(total atom depopulation rate)} \end{aligned} \tag{30}$$

## Calculation in Liouville space

For fully coherent multi-tone light without any spatial decoherence, we can simply use Hilbert-space vector representation, Eq. (18), to calculate the propagation of the light. If the multiple optical tones are only partially coherent, it will be more convenient to use

density-matrix representation to do the calculation in Liouville space. Similarly, we have the mapping from a density matrix to a Liouville vector for the electric field:

$$\boldsymbol{\epsilon}_{\pm} \Longrightarrow |\boldsymbol{\epsilon}_{\pm}). \tag{31}$$

From Eq. (22), the spatial evolution of $\boldsymbol{\epsilon}$ due to alkali-metal atoms is

$$\left(\frac{d\boldsymbol{\epsilon}_{\pm}}{dz}\right)_a = \pm\frac{i}{\hbar}[\boldsymbol{\delta}\mathbf{P}\cdot\boldsymbol{\epsilon}_{\pm} - \boldsymbol{\epsilon}_{\pm}\cdot\boldsymbol{\delta}\mathbf{P}^{\dagger}]. \tag{32}$$

We find the Liouville version of Eq. (32) to be

$$\left(\frac{d}{dz}\right)|\boldsymbol{\epsilon}_{\pm})_a = \mp n_a\mathcal{P}_a|\boldsymbol{\epsilon}_{\pm}), \tag{33}$$

where

$$\mathcal{P}_a = -\frac{i}{n_a\hbar}(\boldsymbol{\delta}\mathbf{P}^{\flat} - \boldsymbol{\delta}\mathbf{P}^{\dagger\sharp}). \tag{34}$$

One can see the equation here is just like the equation of depopulation pumping for alkali-metal atoms.
